# Supplementary material for: On the estimation of inclusion probabilities for weighted analyses of nested case control studies
Source: arXiv:2601.04066 source file (2026-01-07)
Supplement: Supplementary file 1 [file wNCC_supp_material.pdf]

Supplementary Material for

# *"On the estimation of inclusion probabilities for weighted analyses of nested case-control studies"*

## Contents


**1 GAM- versus KM-weights in the NN matching** **2**

**2 Summary Statistics for the Simulation Studies** **4**

**3 Complementary simulation studies** **7**

3.1 GAM-weights for untypical NCCs . . . . . . . . . . . . . . . . . . . . . . . . . . 7

3.2 Estimation of the association between exposures . . . . . . . . . . . . . . . . . 7

**4 Additional results on EPIC ENDO** **13**

# 1 GAM- versus KM-weights in the NN matching

In this first supplementary material we graphically illustrate the fundamental difference between KM- and GAM-weights in replicating the original cohort when a large portion of the population is non-eligible for selection, such as in NN matching. We consider the NN matching setting of Section 3.2 with a single continuous matching variable $M$ and focus on different narrow regions of its distribution to highlight local behavior of the estimated inclusion probabilities.

Figure 1 presents inclusion probabilities estimated using the KM- and GAM-weight approaches for participants in the originating cohort with $D = 0$ and $T \geq 48$ so that variations in inclusion probability are primarily driven by the modeling of $M$.

KM-based probabilities display a highly discontinuous pattern, with values jumping abruptly between 0 and 1. As a result, when a large portion of the sample is ineligible for selection, KM weights cannot generalize beyond the eligible population. In contrast, GAM-based probabilities vary smoothly across $M$, as they are derived from a flexible model that accounts for gradual changes in inclusion likelihood. This smooth estimation enables GAM weights to borrow information from individuals with similar—but not identical—profiles, thereby producing a pseudo-population that more accurately reflects the full originating cohort.

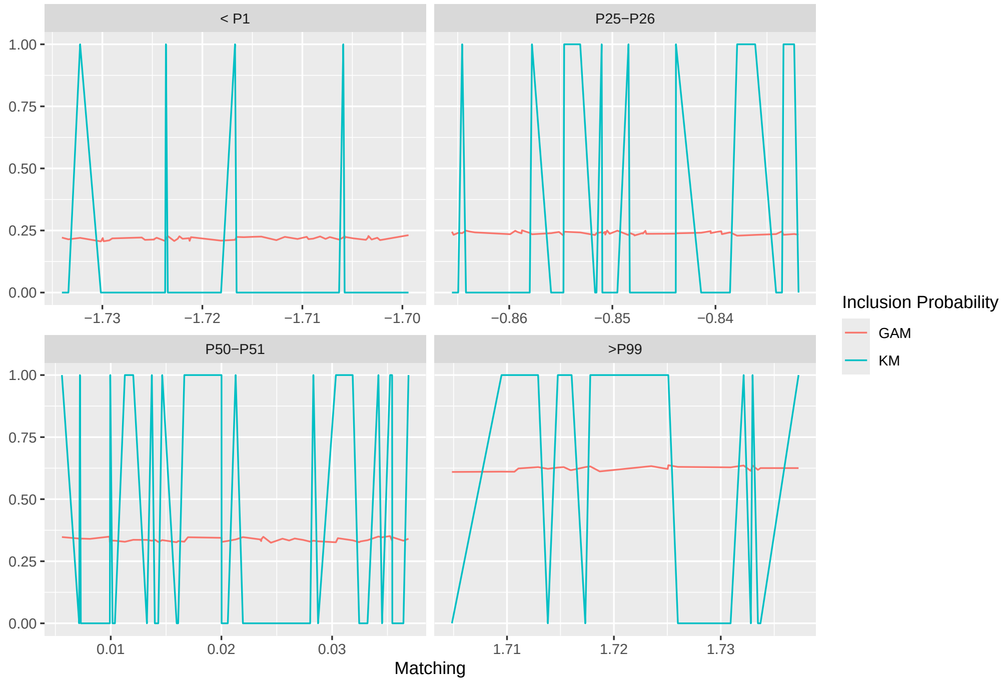


Figure 1: Illustration of the differences between inclusion probabilities estimated using GAM-weights and KM-weights in the nearest neighbor (NN) matching setting of Section 3.2 of the paper. The $x$-axis represents standardized values of $M$, and each panel zooms into a narrow region of its distribution—specifically below the 1st percentile, between the 25th and 26th percentiles, between the 50th and 51st percentiles, and above the 99th percentile (with "P" denoting percentiles).

## 2 Summary Statistics for the Simulation Studies

In this supplementary material we present summary statistics for the three target estimands based on the simulation settings described in Section 3 of the paper. For each setting, we report the mean and standard error of estimates obtained from the full cohort and from the nested case-control (NCC) sample using the different versions of KM- and GAM-weights considered. We additionally indicate statistical differences relative to the full cohort estimates. Tables 2–2 summarize results under different conditions: comparisons between caliper and nearest-neighbor (NN) matching (Table 2), scenarios with interactions between matching variables that affect event risk (Table 2), and settings where some matching factors can be omitted (Table 2).

| | Caliper Matching | NN Matching |
|---|---|---|
| **Panel A: Log-HR ($\alpha_b$)** | | |
| Full Cohort | 0.692 (0.007) | 0.692 (0.007) |
| Cond. Log. Reg. | 0.691 (0.012) | 0.693 (0.013) |
| KM | 0.693 (0.010) | **0.512** (0.008) |
| GAM | 0.692 (0.010) | 0.692 (0.012) |
| **Panel B: Conditional Survival** | | |
| Full Cohort | 0.121 (0.002) | 0.121 (0.002) |
| KM | 0.121 (0.002) | **0.343** (0.004) |
| GAM | 0.121 (0.002) | 0.121 (0.002) |
| **Panel C: Linear Regression Coefficient ($\theta$)** | | |
| Full Cohort | 0.315 (0.003) | 0.315 (0.003) |
| KM | 0.314 (0.008) | **0.348** (0.005) |
| GAM | 0.314 (0.008) | 0.315 (0.008) |

Table 1: Summary Statistics from simulation results in the case of nearest-neighbor matching versus caliper matching (see Figure 3 of the paper). Reported values are means with standard errors in parentheses. Values in bold are significantly different from the Full Cohort estimates at the 95% confidence level.

| | $\alpha_{\text{MSNP}} = 0$ | | $\alpha_{\text{MSNP}} = 0.69$ | |
|---|---|---|---|---|
| | $\alpha_{\text{M1M2}} = 0$ | $\alpha_{\text{M1M2}} = 0.69$ | $\alpha_{\text{M1M2}} = 0$ | $\alpha_{\text{M1M2}} = 0.69$ |
| **Panel A: Log-HR** ($\alpha_b$) | | | | |
| Full Cohort | 0.692 (0.012) | 0.695 (0.014) | 0.696 (0.013) | 0.692 (0.015) |
| Cond. Log. Reg. | 0.692 (0.017) | 0.695 (0.018) | 0.696 (0.019) | 0.692 (0.020) |
| GAM | 0.698 (0.029) | **0.710** (0.025) | **0.703** (0.029) | **0.713** (0.028) |
| GAM with InterM | 0.697 (0.029) | 0.698 (0.024) | 0.701 (0.028) | 0.693 (0.027) |
| KM | 0.697 (0.029) | 0.698 (0.024) | 0.700 (0.028) | 0.694 (0.027) |
| **Panel B: Conditional Survival** | | | | |
| Full Cohort | 0.027 (0.001) | 0.030 (0.002) | 0.033 (0.002) | 0.017 (0.001) |
| GAM | 0.028 (0.002) | **0.032** (0.002) | **0.034** (0.002) | **0.017** (0.001) |
| GAM with InterM | 0.028 (0.002) | 0.030 (0.002) | 0.033 (0.002) | 0.017 (0.001) |
| KM | 0.028 (0.002) | 0.030 (0.002) | 0.033 (0.002) | 0.017 (0.001) |
| **Panel C: Linear Regression Coefficient** ($\theta$) | | | | |
| Full Cohort | 0.315 (0.003) | 0.315 (0.003) | 0.315 (0.003) | 0.315 (0.003) |
| GAM | 0.313 (0.011) | **0.306** (0.011) | **0.310** (0.014) | **0.303** (0.014) |
| GAM with InterM | 0.314 (0.011) | 0.313 (0.015) | 0.315 (0.014) | 0.316 (0.015) |
| KM | 0.315 (0.011) | 0.313 (0.015) | 0.315 (0.014) | 0.316 (0.015) |

Table 2: Summary Statistics from simulation results in the presence of interactions with $\alpha_M = 0$ (see Figure 4 of the paper). Reported values are means with standard errors in parentheses. Values in bold are significantly different from the Full Cohort estimates at the 95% confidence level.

| | M∼Z | M∼V | M∼W |
|---|---|---|---|
| **Panel A: Log-HR ($\alpha_b$)** | | | |
| Full Cohort | 0.692 (0.001) | 0.692 (0.001) | 0.692 (0.001) |
| Cond. Log. Reg. | 0.690 (0.001) | 0.690 (0.001) | 0.691 (0.001) |
| KM | 0.693 (0.001) | 0.691 (0.001) | 0.693 (0.001) |
| GAM | 0.693 (0.001) | 0.691 (0.001) | 0.692 (0.001) |
| KM wo M | 0.693 (0.001) | **0.704** (0.001) | **0.702** (0.001) |
| GAM wo M | 0.693 (0.001) | **0.713** (0.001) | **0.708** (0.001) |
| **Panel B: Conditional Survival** | | | |
| Full Cohort | 0.101 (0.000) | 0.121 (0.000) | 0.121 (0.000) |
| KM | 0.101 (0.000) | 0.121 (0.000) | 0.121 (0.000) |
| GAM | 0.101 (0.000) | 0.121 (0.000) | 0.121 (0.000) |
| KM wo M | 0.101 (0.000) | **0.124** (0.000) | 0.120 (0.000) |
| GAM wo M | 0.101 (0.000) | **0.117** (0.000) | **0.115** (0.000) |
| **Panel C: Linear Regression Coefficient ($\theta$)** | | | |
| Full Cohort | 0.315 (0.000) | 0.315 (0.000) | 0.315 (0.000) |
| KM | 0.315 (0.001) | 0.315 (0.001) | 0.314 (0.001) |
| GAM | 0.315 (0.001) | 0.315 (0.001) | 0.314 (0.001) |
| KM wo M | 0.315 (0.001) | 0.316 (0.001) | **0.320** (0.001) |
| GAM wo M | 0.315 (0.001) | 0.314 (0.001) | **0.319** (0.001) |

Table 3: Summary Statistics from simulation results illustrating that some matching factors can be ignored (see Figure 5 of the paper). Reported values are means with standard errors in parentheses. Values in bold are significantly different from the Full Cohort estimates at the 95% confidence level.

# 3 Complementary simulation studies

In this supplementary material we present additional results from simulation studies. First, we illustrate the performance of weighted analyses based on GAM-weights defined in Equation 5 of the paper within the context of untypical NCC studies. We then focus on estimating the association between exposures and highlight limitations of weighted analyses in the common situation where follow-up times are short and weights are large for some controls selected in the NCC.

## 3.1 GAM-weights for untypical NCCs

We illustrate the performance of GAM-weights in the setting of untypical NCCs with $\pi_1 = 0.5$ and caliper matching. For comparison, results are also presented in the setting of typical NCCs with $\pi_1 = 1$. The size of the originating cohort is set to $10^5$ and $2 \times 10^5$ in the typical and untypical settings, respectively, to make the average number of cases selected in the NCC studies similar and to facilitate the comparison of results across the two settings. We generate synthetic cohorts with a single matching factor $M = M_1$ and parameters $\alpha_{M_1 M_2}$ and $\alpha_{M \cdot X_a}$ both set to 0. We consider two settings, namely $\{\rho_{MX_a} = 0.2, \alpha_{M_1} = \log(2)\}$, and $\{\rho_{MX_a} = 0, \alpha_{M_1} = 0\}$, which corresponds to settings where $M$ behaves as $\mathbf{W}$ (i.e., influences both $\mathbf{X}$ and $Y$), and $\mathbf{Z}$ (i.e., influences neither $\mathbf{X}$ nor $Y$) [1], respectively. Results obtained in these two settings are presented in Figures 2 and 3, respectively, for the particular choice $\gamma_{MX_b} = 0$, $\alpha_a = 0$ and $\alpha_b = \log(2)$. Other values of these parameters lead to similar results, which are omitted.

The Results of the analyses of untypical and typical NCC studies are similar: KM-weights (or more precisely HT-weights in the case of untypical NCC studies) and GAM-weights perform similarly in the setting we consider here. Ignoring the matching factor when computing GAM-weights lead to biased estimates when the matching factor influences both the exposure and disease risk (Figure 2), but not when it influences neither (Figure 3).

## 3.2 Estimation of the association between exposures

As mentioned in the main article, concerns have been raised in the literature about the use of inverse-probability weighting to infer the distribution of exposures stoersamuelsen2016. In particular, extreme weights can be assigned to controls with short follow-up and can strongly inflate variance. Here, we present results from simulation studies designed to illustrate this limitation. We focus on the setting of typical NCCs ($\pi_1 = 1$) with caliper matching based on a single matching factor $M_1$. By varying the values of parameters $u_0$ and $u_1$, we consider situations with low censoring ($u_0 = 20$ and $u_1 = 50$), moderate censoring ($u_0 = 20$

[1] See in Figure 8 in the paper

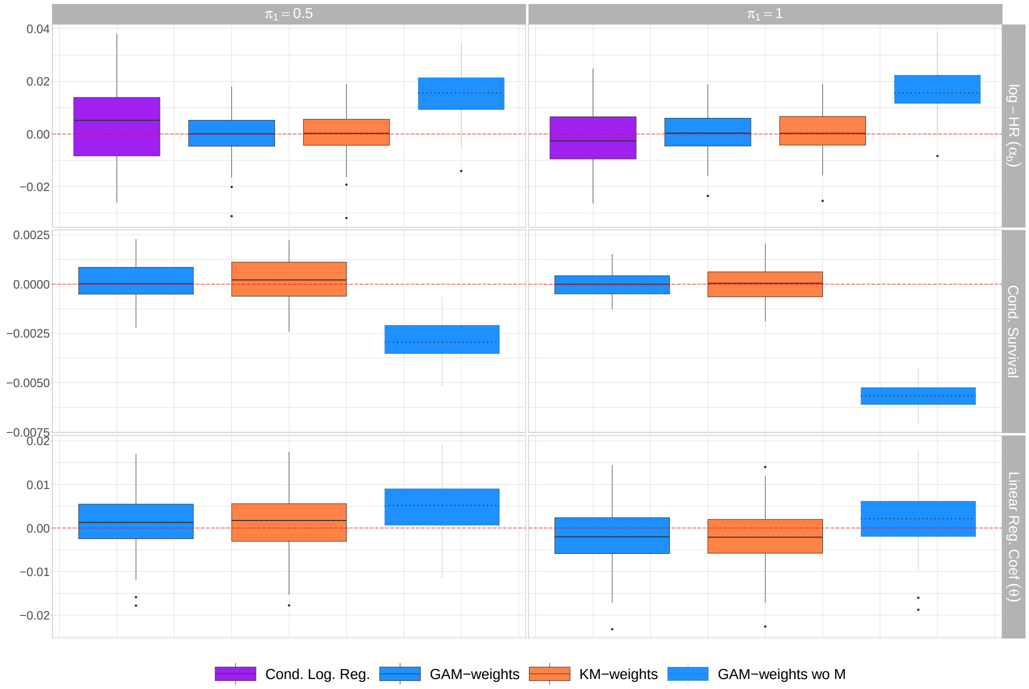


Figure 2: Illustration of the performance of GAM-weights for untypical NCC studies, when the matching factor influences both the exposure and the disease risk. Each plot represents the observed distribution of the differences between the estimate produced by one particular type of analysis and the estimate obtained on the full cohort over 50 replicates.

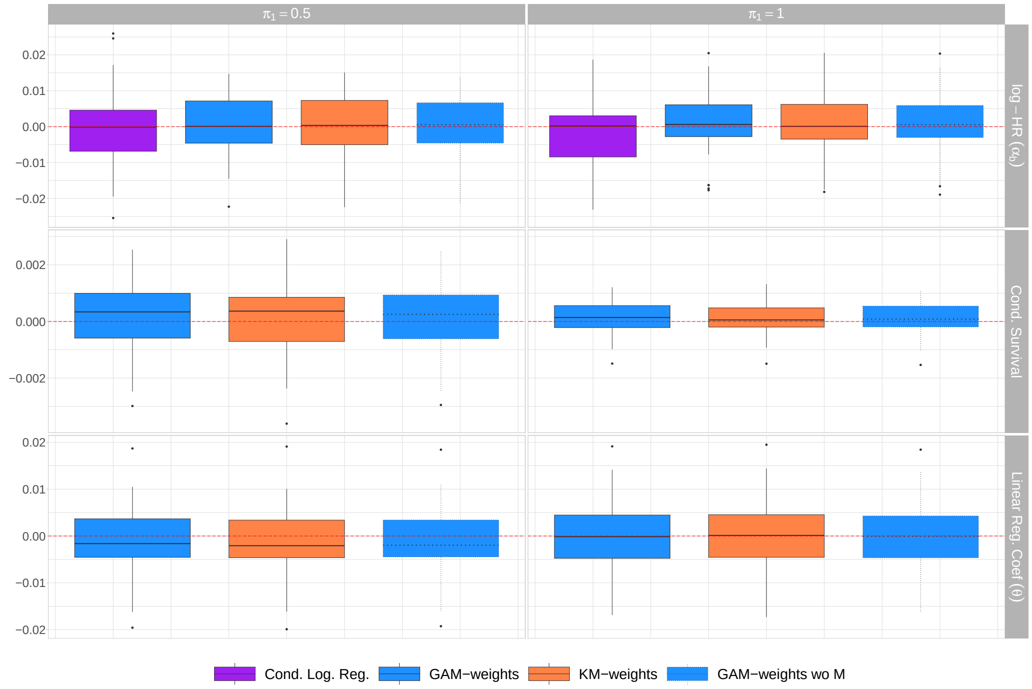


Figure 3: Illustration of the performance of GAM-weights for untypical NCC studies, when the matching factor influences neither the exposure nor the disease risk. Each plot represents the observed distribution of the differences between the estimate produced by one particular type of analysis and the estimate obtained on the full cohort over 50 replicates.

and $u_1 = 30$), and high censoring ($u_0 = 0$ and $u_1 = 30$). This allows us to assess the performance of weighted analyses in situations where follow-up can be short, and weights large, for some controls selected in the NCC study. Following the observation we made in the last paragraph of appendix 1.3 in the paper, we further make parameters $\alpha_a$ and $\alpha_b$ vary to assess the performance of the different approaches in situations where the NCC design leads to ($i$), no collider bias ($\alpha_a = \log(2)$ and $\alpha_b = 0$), ($ii$), moderate collider bias ($\alpha_a = 0$ and $\alpha_b = \log(2)$), and ($iii$) strong collider bias ($\alpha_a = \log(2)$ and $\alpha_b = \log(2)$), for the estimation of the association between $X_a$ and $X_b$. Figures 4 and 5 present the results for $\alpha_{M_1} = \log(2)$ when the association does not depend on $M_1$ ($\gamma = 0$) and when it does depend on $M_1$ ($\beta = 0$), respectively.

As in the main article, we consider weighted analyses based on GAM- and KM-weights. For comparison, we further consider three types of unweighted analyses: the unweighted analysis of the full NCC study, of the controls of the NCC study, and of a random subset of the cohort of equal size to that of the NCC study. This later comparison allows us to illustrate possible limitations of weighted analyses in terms of variance of the estimates, especially where controls with short follow-up are selected in the NCC study. We also consider two additional versions of GAM-weights: ($i$), the thresholded version of the standard GAM-weights, where weights larger than 100 are capped to 100, and ($ii$), a version based on estimates of $P(S = 1|M)$, thus ignoring variables $(D, T)$. These versions are referred to as "GAM-weights thresh." in and "GAM-weights w/o $(T, D)$", respectively, in Figures 4 and 5.

First consider the case where the association between $X_a$ and $X_b$ does not depend on $M$ (Figure 4). In the absence of collider bias, all approaches produce unbiased estimates of the coefficient of the linear regression of $X_b$ on $X_a$. However, weighted analyses based on KM- or GAM-weights produce estimates with larger variance, especially in the high censoring setting, where controls with short follow-ups typically receive large weights. Thresholded weights generally improve the performance of weighted analyses, although some moderate bias is observed in the setting with highest censoring. GAM-weights based on the estimation of $P(S = 1 \mid M)$, which ignore $T$ and $D$, yield unbiased estimates with empirical variances comparable to those obtained from unweighted analyses of fully random subsamples, thereby confirming their optimality in the absence of collider bias. The performance of weighted analyses is generally unaffected by collider bias, except when weights that ignore $T$ and $D$ are used, in which case the resulting bias is comparable in magnitude to that observed in the unweighted analysis of the NCC study.

Patterns are mostly similar when the association between $X_a$ and $X_b$ depends on $M$ (Figure 5). The main difference is that the unweighted analyses of the full NCC study or of the controls of the NCC study lead to biased estimates of the association between $X_a$ and $X_b$, even in the absence of collider bias. This is because we consider the situation

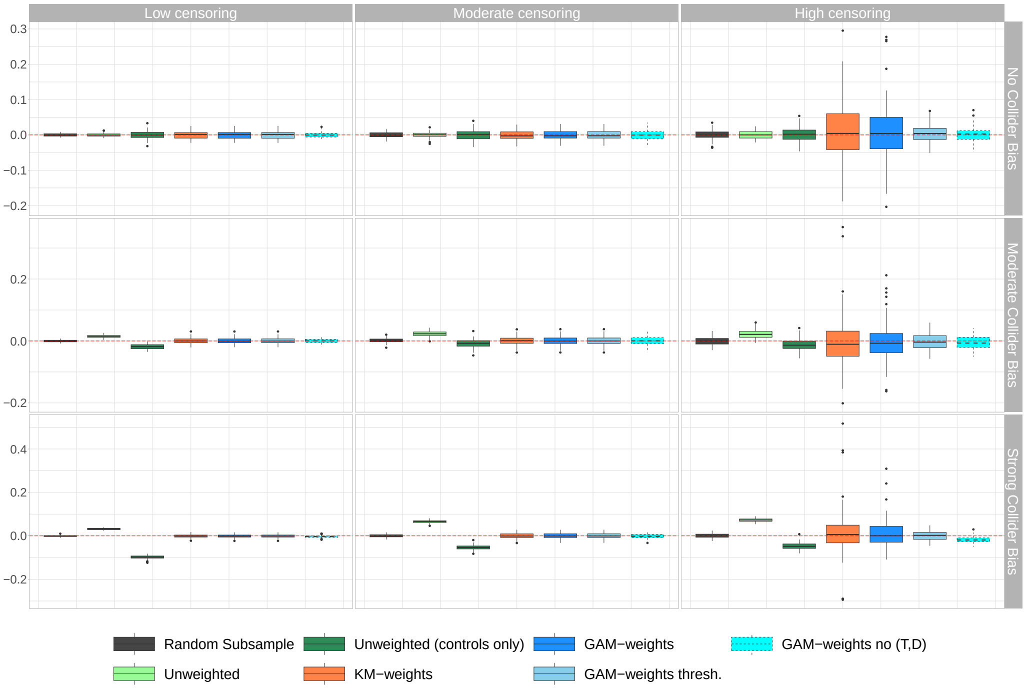


Figure 4: Results for the estimation of the marginal association between $X_a$ and $X_b$ in the case where their association does not depend on $M_1$ ($\gamma = 0$). Each plot represents the observed distribution of the differences between the estimate produced by one particular type of analysis and the estimate obtained on the full cohort over 100 replicates.

where $M$ is associated with the outcome $Y$ ($\alpha_M = \log(2)$), so that the distribution of $M$ is shifted to the right in the NCC study compared to the full cohort. Therefore, because $E(X_b|X_a, M) = \gamma M X_a$ with $\gamma > 0$, the marginal association between $X_a$ and $X_b$ is larger in the NCC study compared to the full cohort. Another difference is that weighted analyses based on thresholded GAM-weights tend to slightly overestimate the association between $X_a$ and $X_b$ when censoring is high, regardless of the strength of collider bias, while this was not the case on Figure 4.

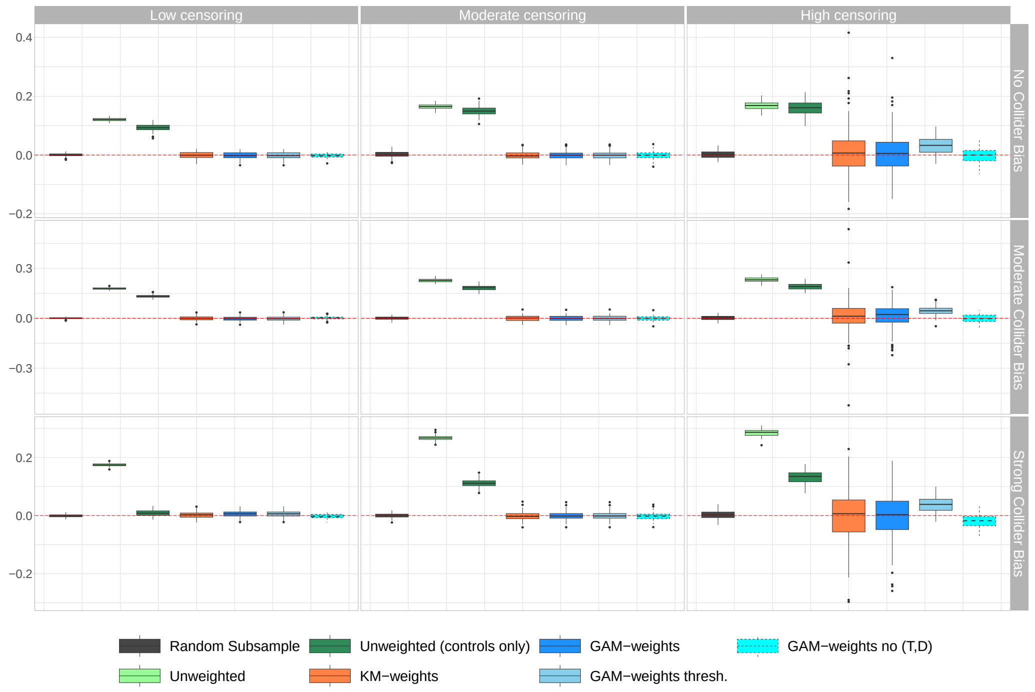


Figure 5: Results for the estimation of the marginal association between $X_a$ and $X_b$ in the case where in the case where their association depends on $M_1$ ($\gamma > 0$ and $\beta = 0$). Each plot represents the observed distribution of the differences between the estimate produced by one particular type of analysis and the estimate obtained on the full cohort over 100 replicates.

# 4 Additional results on EPIC ENDO

Here we present results from our analyses of the EPIC ENDO study. Figure 6 shows the distribution of the four types of weights among the controls of EPIC ENDO, as well as the correlations between these weights estimated in the controls of the study. Figure 7 presents Kaplan-Meier estimates of the survival function of endometrial cancer derived from the originating cohort, the eligible sub-population, and various weighted analyses of the EPIC ENDO NCC study. Finally, Figure 8 presents a heatmap of the estimated correlations between BMI and the 117 metabolites. In particular, it highlights the strong similarity between the estimates from the unweighted analysis of the controls and those from the weighted analysis using thresholded GAM-weights.

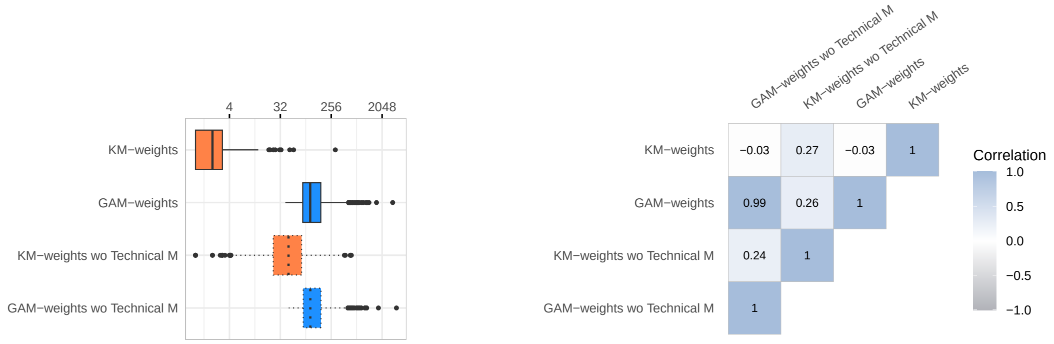


Figure 6: Distribution of the weights in the controls of EPIC ENDO

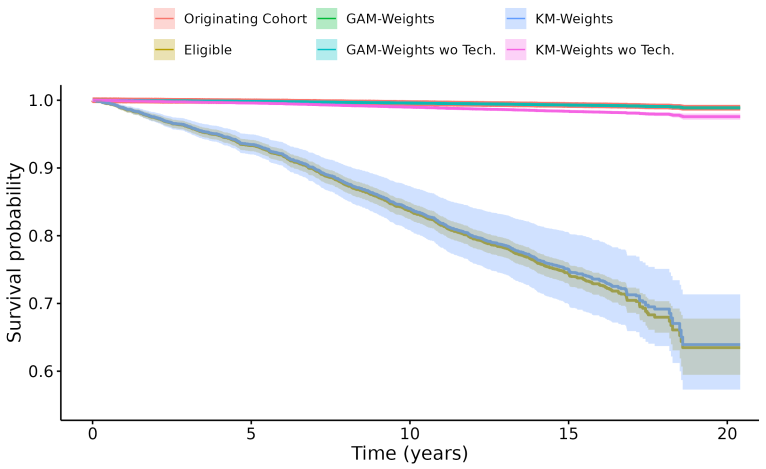


Figure 7: Kaplan-Meier estimates of the (unconditional) survival probability of endometrial cancer in EPIC.

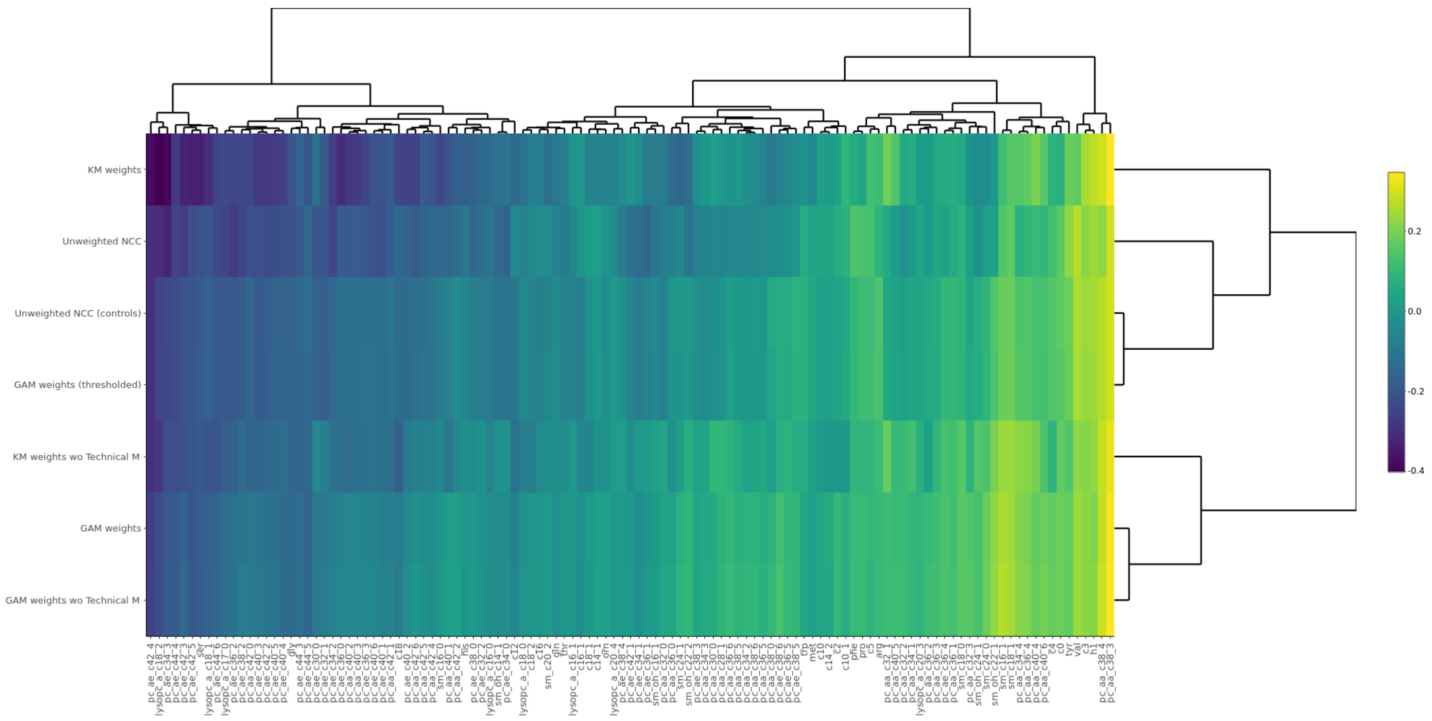


Figure 8: Heatmap of the correlation between BMI and the 117 metabolites measured in EPIC ENDO, depending on the weighted or unweighted analysis considered
